# Supplementary material for: Black Swan: Abductive and Defeasible Video Reasoning in Unpredictable Events
Source: arXiv:2412.05725 source file (2025-04-07)
Supplement: Supplementary file 1 [file PC-crop.pdf]

## Welcome!

Welcome to this task! Please being by reading the full instructions and the guidelines.

**Full Instructions** (Expand/Collapse)

# Task Instructions

Thanks for participating in this task. Your goal is to describe a very short video clip (can be a small part of a longer video) to the best of your ability.

1. **Step 1:** First, watch the video carefully and think about the scene, the objects and people, and their actions.
2. **Step 2:** Next, describe the video in a few sentences. You must write at least 25 words, but longer descriptions are welcome.
3. **Step 3:** Check to ensure that you are not making any *assumptions* about the contents in the video, and that your description contains all aspects of the scene.

# Example 1

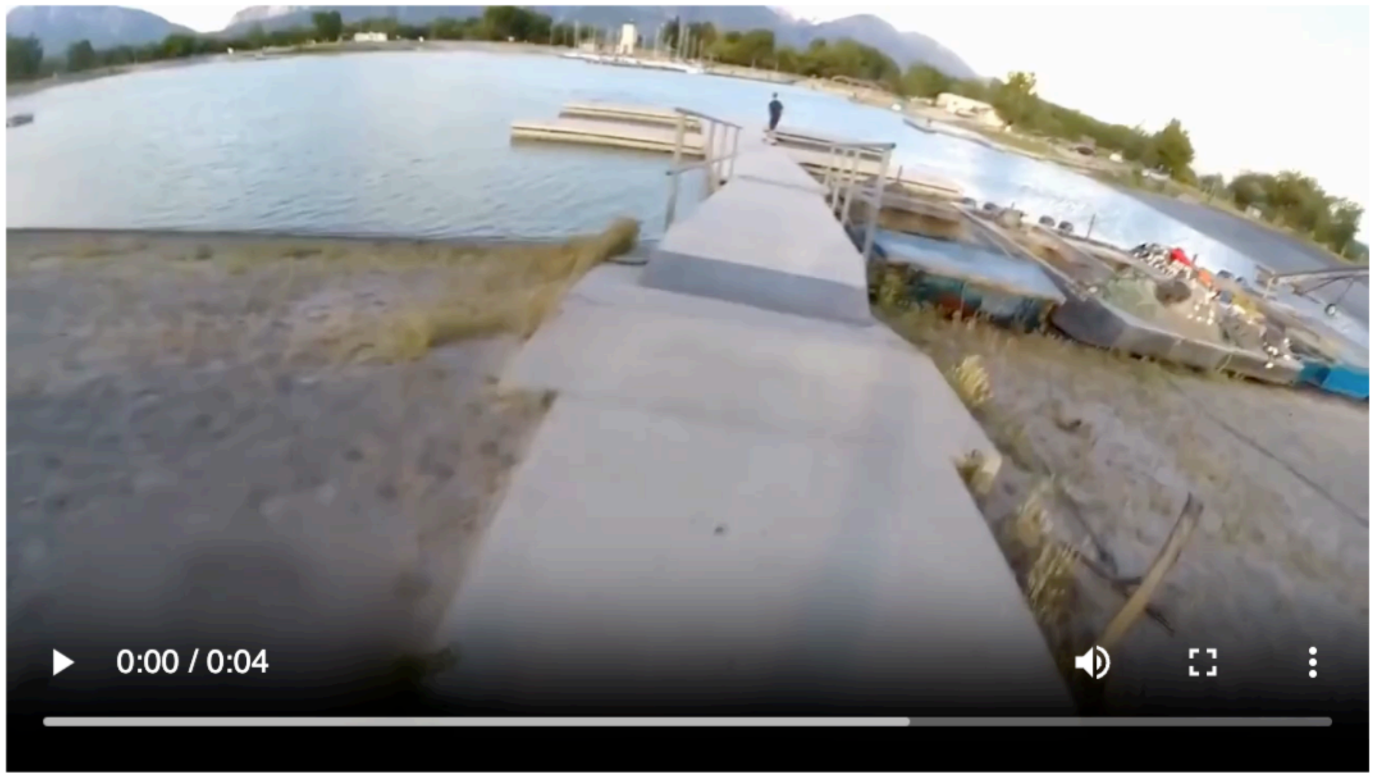


Watch this clip and describe everything about the contents of the video:

A person is walking towards a body of water, may be a lake on a board walk with a fishing stick. Then, the person sees a silver sedan moving towards the water on his left. The person steps off the boardwalk towards the car hastily. The video is in the perspective of the person walking.

## Example 2

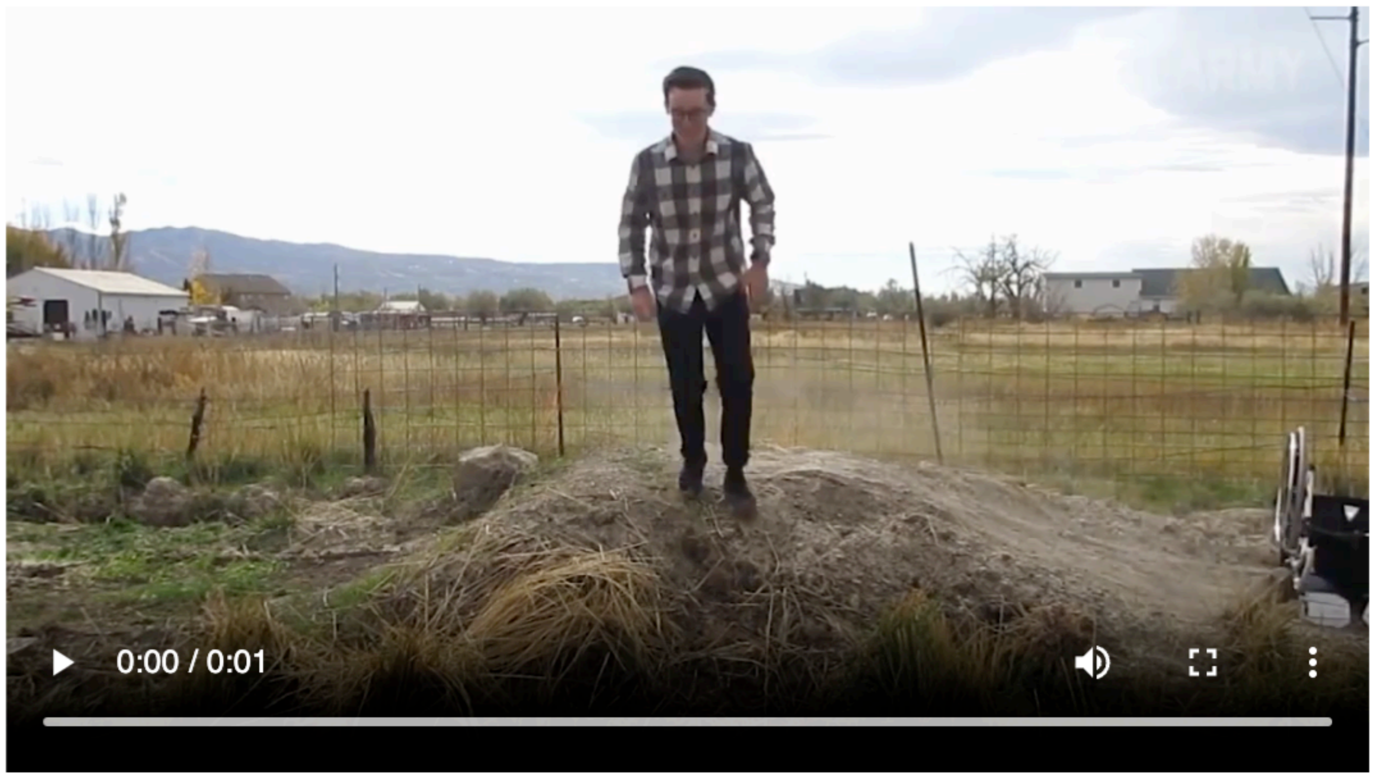


Watch this clip and describe everything about the contents of the video:

A man walks down a small mud hill towards the camera. There appears to be an upside-down wheelchair to the right of the scene. The secene is set in a farm-like area, with a shed in the back and mostly grassy fields.

## Example 3

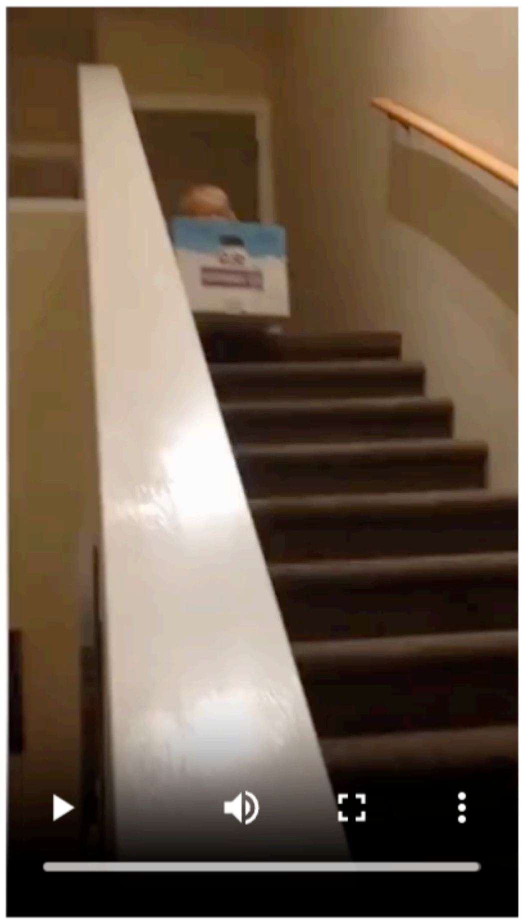

Watch this clip and describe everything about the contents of the video:

Two kids are sitting in a cardboard box, and they have started going down the stairs of the house while riding in the box. The camera is pointed looking up towards the stairs.

# Guidelines:

- **Objects** - **Describe the objects present in the scene and the state/location of the objects.**
- **People** - **Identify and describe the people in the video (eg. young child, old lady...).**
- **Actions** - **Describe the movements or actions in the video.**
- **Scene** - **Descibe the scene and setting, and where the camera is pointed.**

# Task: Describe the events in this video

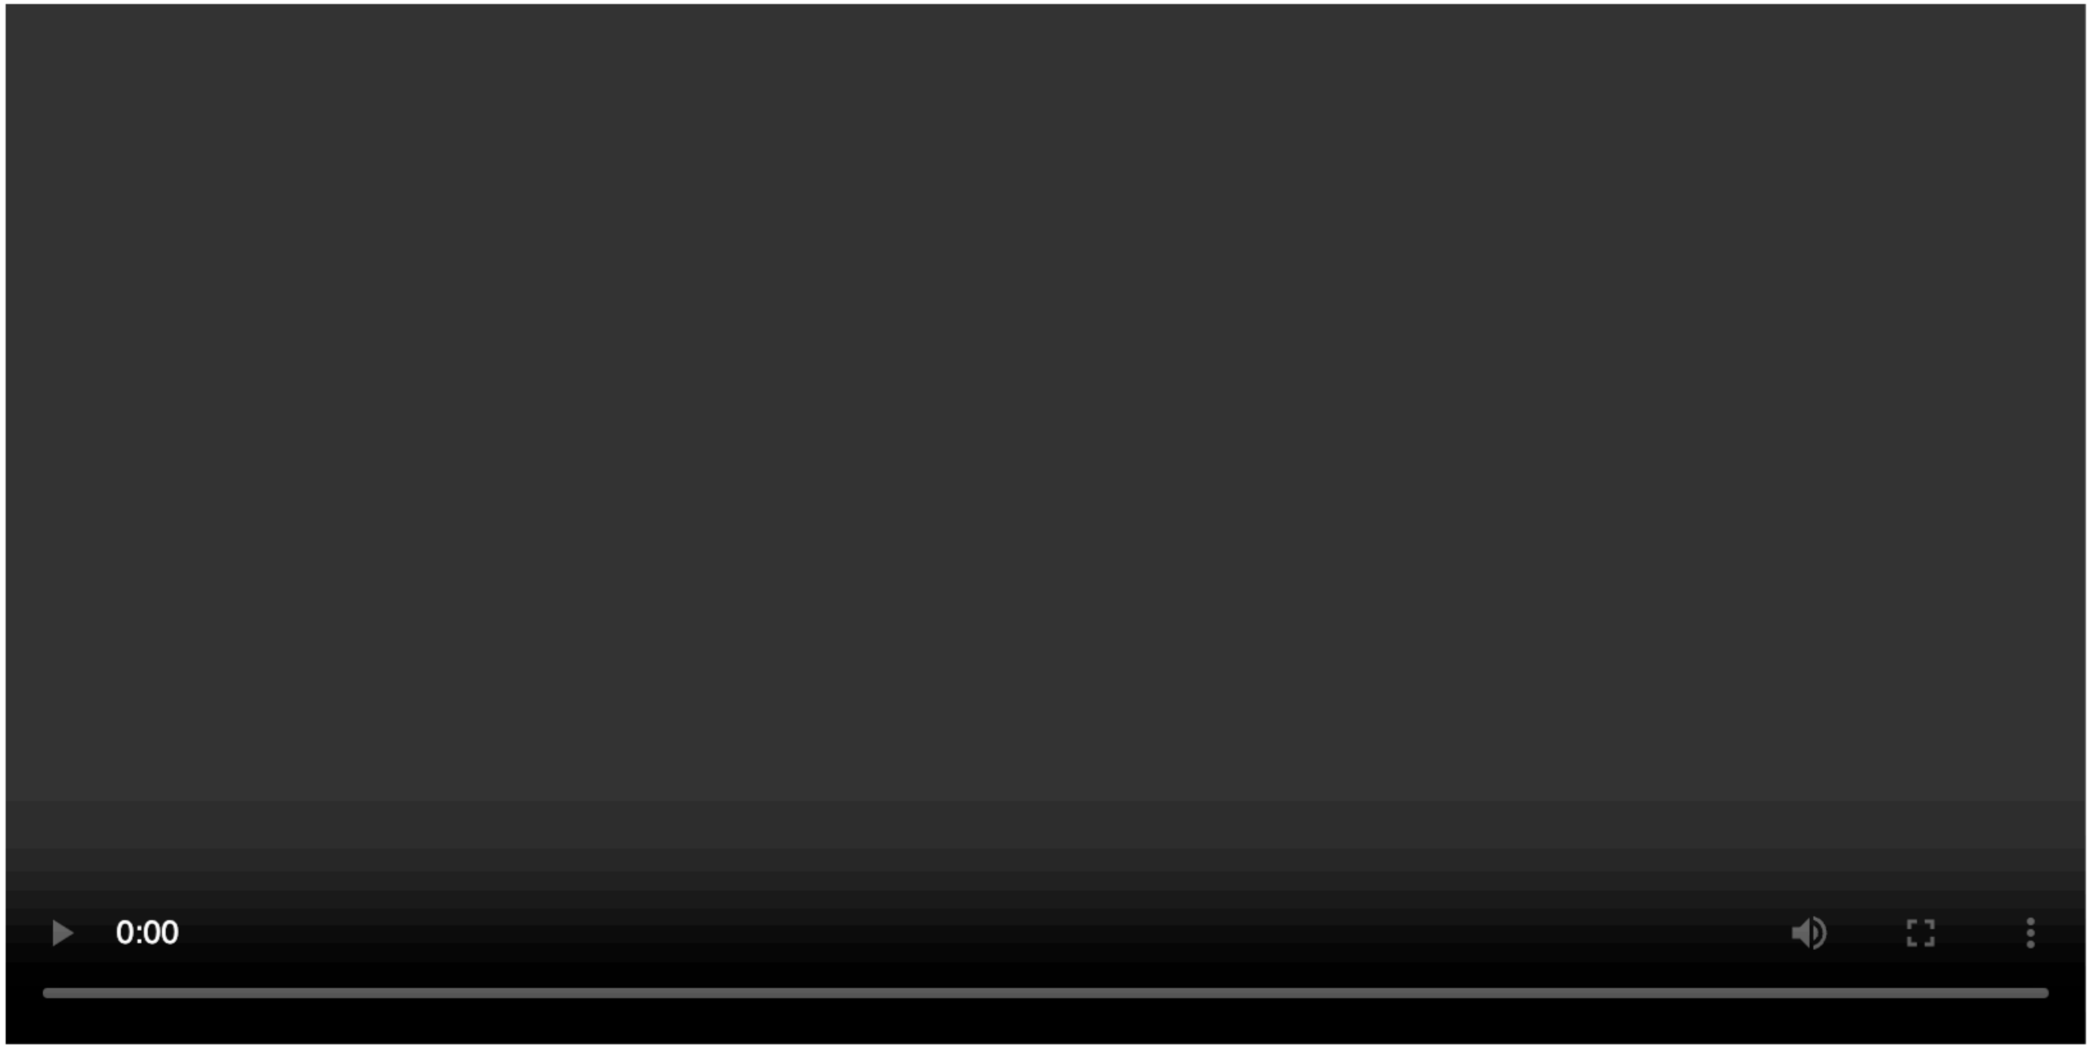


Watch this clip and describe what is happening in the video.

**Please check that your description contains information about:**

Scene Objects People Actions

Submit

## Welcome!

Welcome to this task! Please being by reading the full instructions and the guidelines.

**Full Instructions** (Expand/Collapse)

# Task Instructions

Thanks for participating in this task. Your goal is to **describe the differences** between two short video clips, the beginning and end of a video. Please note that the middle of the clip is hidden on purpose, so you should not make any assumptions about the contents of what happend in the middle.

1. **Step 1:** First, watch both the beginning and the end video carefully and think about the scene, the objects and people, and their actions.
2. **Step 2:** Next, describe the differences you observe in the scene, objects, people and actions between the beginning and end of the video (in at least 15 words).
3. **Step 3:** Check to ensure that you are not making any *assumptions* about the contents in the videos, and that your description contains all aspects of the scene.

# Example 1

**Beginning:**

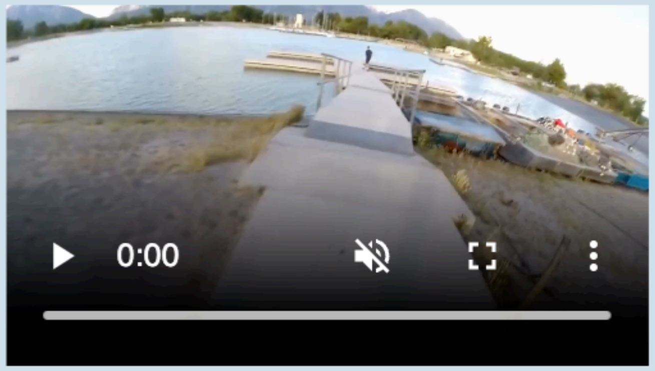


**Middle (Hidden)**

**End:**

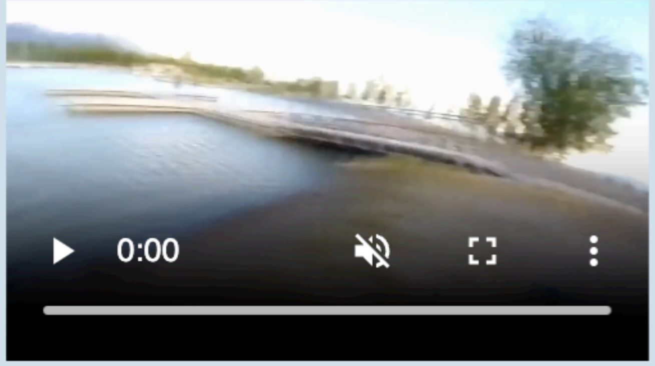


What are the differences in the scene between the beginning and the end?

In the beginning the car is on the beach whereas in the end, the car is in the water.

## Example 2

| Beginning: | Middle (Hidden) | End: |
| --- | --- | --- |
| 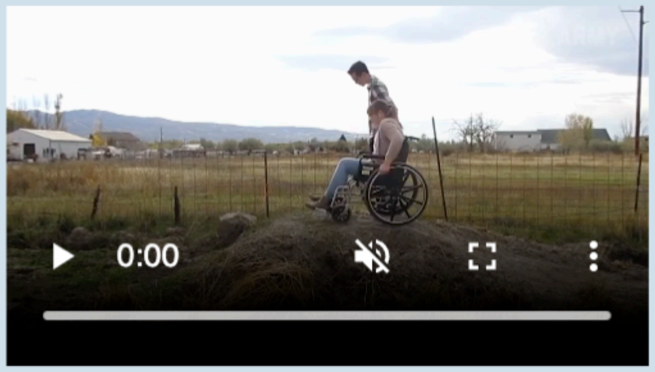 | | 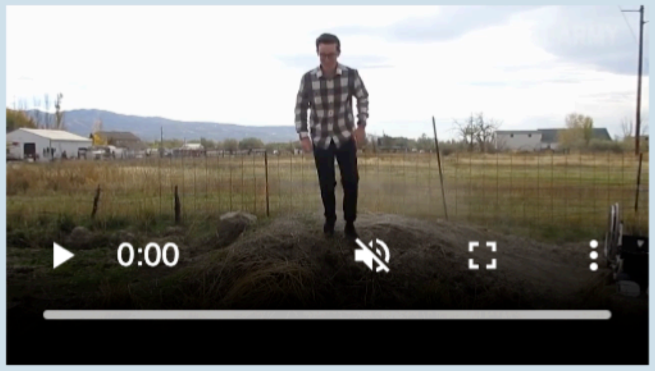 |

What are the differences in the scene between the beginning and the end?

> In the beginning, the man and the woman in the wheelchair are on top of a mud hill, whereas in the end, the wheelchair is upside down on the right of the frame, and the woman is no longer visible.

## Example 3

| Beginning: | Middle (Hidden) | End: |
| --- | --- | --- |
| 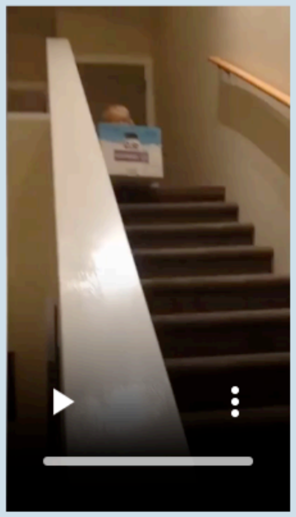 | | 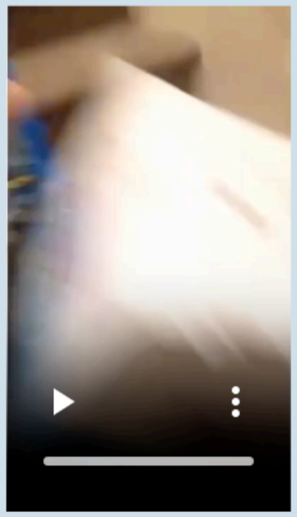 |

What are the differences in the scene between the beginning and the end?

> The two kids are in a box on the top of the stairs in the beginning. In the end, the kids are on the floor at the end of the staircase, and both look like they took a fall. The box seems to be upside down.

# Guidelines:

- **Objects** - **Describe the changes to the objects present in the scene and the state/location of the objects.**
- **People** - **Identify and describe what happened to the people in the video.**
- **Actions** - **Describe the movements or actions in the video (but do not make assumptions about what happened in the middle).**
- **Scene** - **Describe the scene and setting, and where the camera is pointed, before and after, if changed.**

# Task: Multiple Choice Question Answering

**Beginning:**

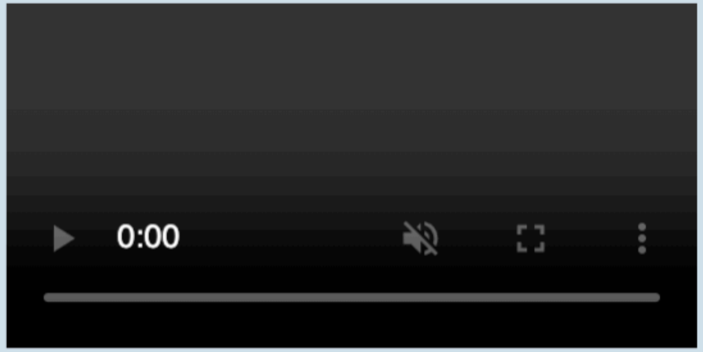


**Middle (Hidden)**

**End:**

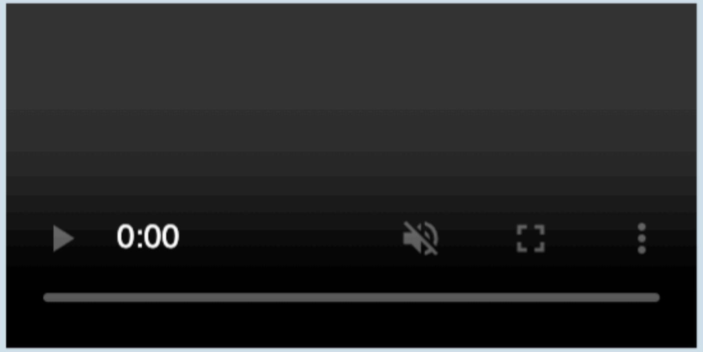


What are the differences in the scene between beginning and end?

Please ensure you have read the examples in the instructions, to understand what is expected, before proceeding.

**Please check that your description contains information about:**

Scene Objects People Actions

Submit
