# Supplementary material for: Black Swan: Abductive and Defeasible Video Reasoning in Unpredictable Events
Source: arXiv:2412.05725 source file (2025-04-07)
Supplement: Supplementary file 2 [file VARFigures-egs-crop.pdf]

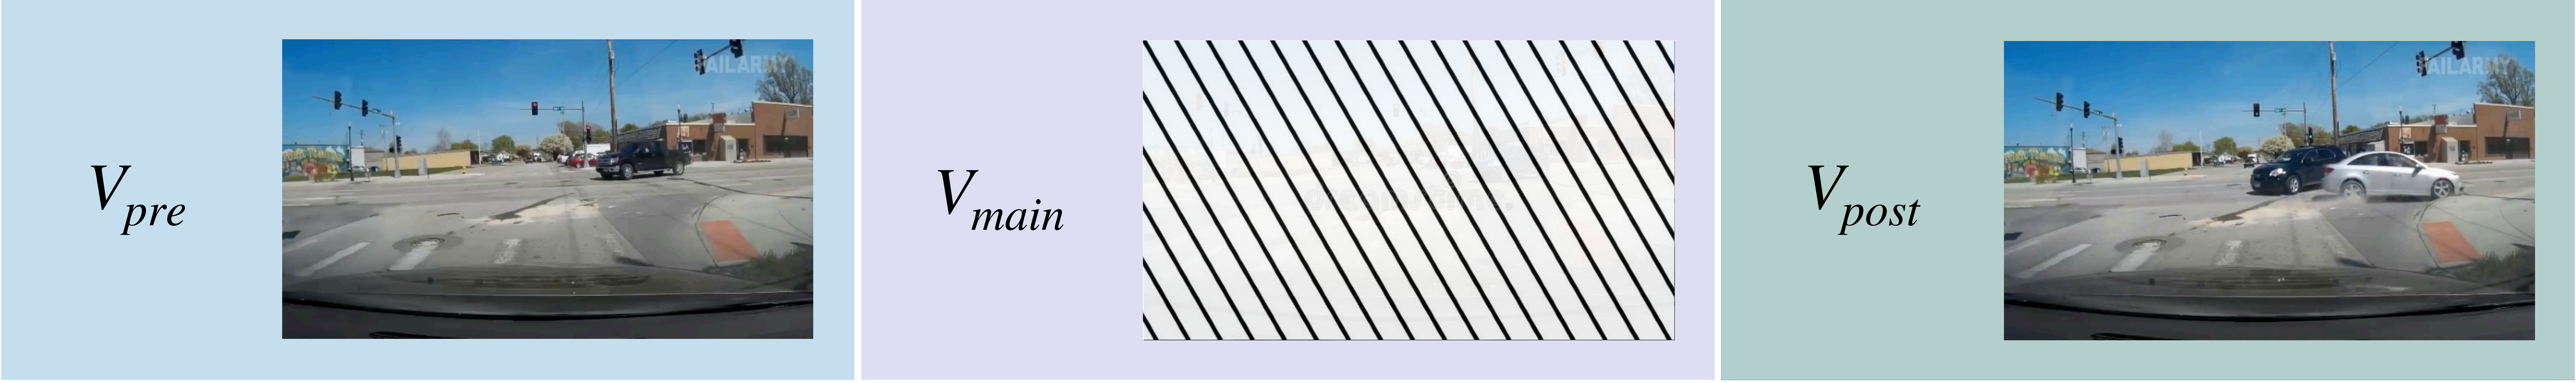


**Question: Explain what could have happened in between.**

A. A car from the left comes speeding through almost hitting the black car.
B. The oncoming car speeds through a red light
C. The black suv turns and runs into the car that is filming

**GT Ans: A**

**GPT-4o Answer:**

Reason:

Step 1: In the beginning frames, a black SUV is making a left turn at an intersection,
Step 2: The SUV completes its turn without hitting anything visible,
Step 3: In the end frames, a silver car is seen, indicating a sudden appearance,
Step 4: The silver car seems to have come from the direction of the left, suggesting it sped through
Step 5: There is no visual evidence of a collision with the filming car

Answer: A. ✅

$V_{pre}$

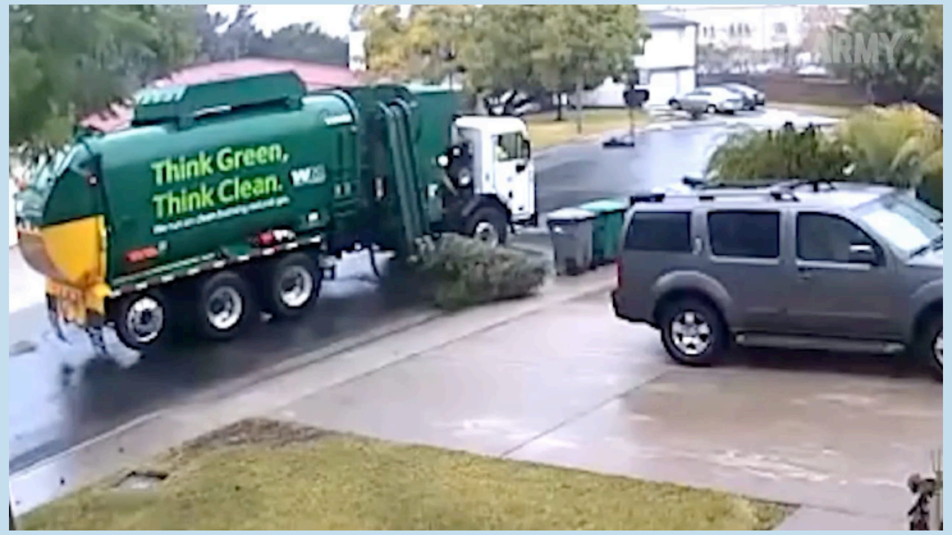


$V_{main}$

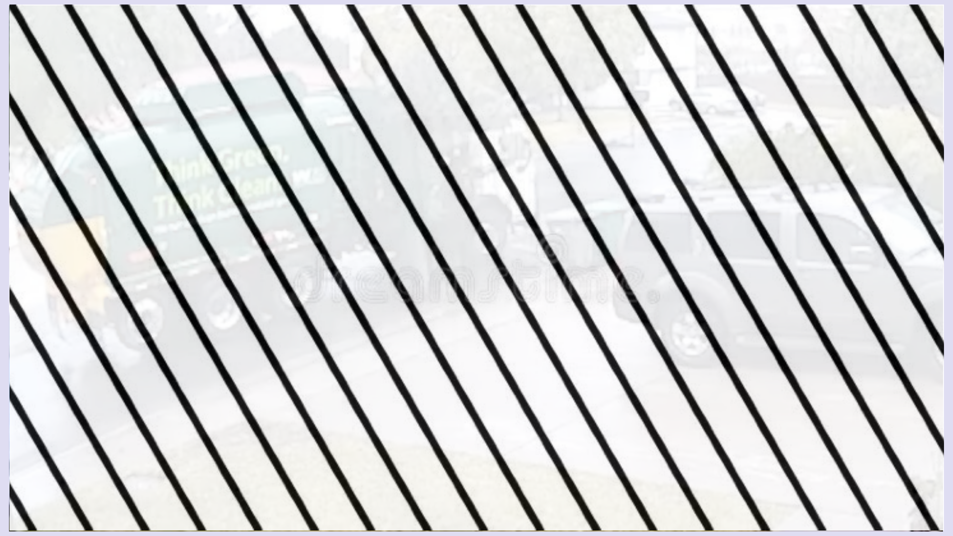

$V_{post}$

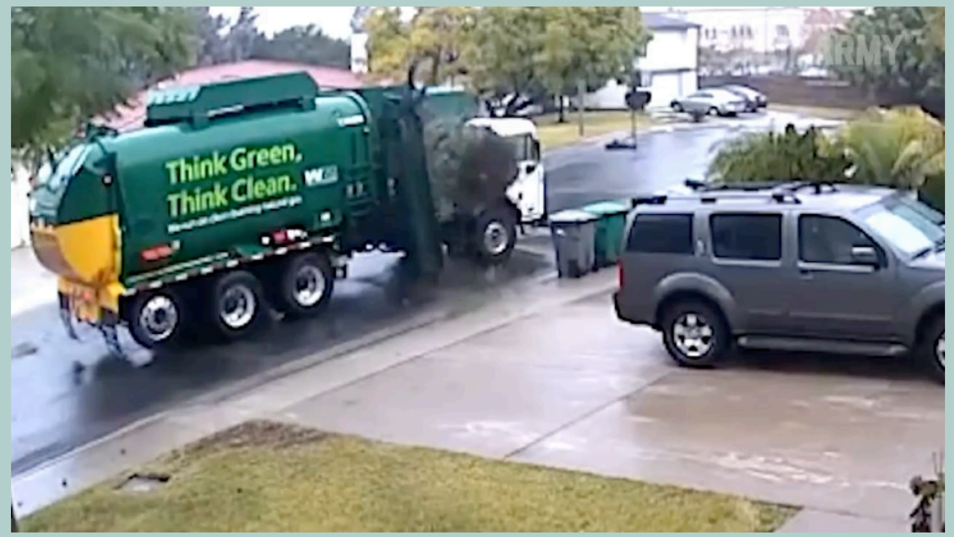


**Question: Explain what could have happened in between.**

A. The garbage truck will park on the side of the road and collect trash from a green bin.
B. The truck will malfunction, dropping the tree on the ground.
C. The tree will be sent flying in the air and damage a nearby car.

**GT Ans: B**

**GPT-4o Answer:**

Reason:

Step 1: The initial frames show a garbage truck lifting a tree,
Step 2: The final frames show the tree being held higher by the truck,
Step 3: There is no visible damage to the surrounding area,
Step 4: Green bins are present, suggesting routine collection

Answer: A. The garbage truck will park on the side of the road and collect trash from a green bin. ❌

$V_{pre}$ 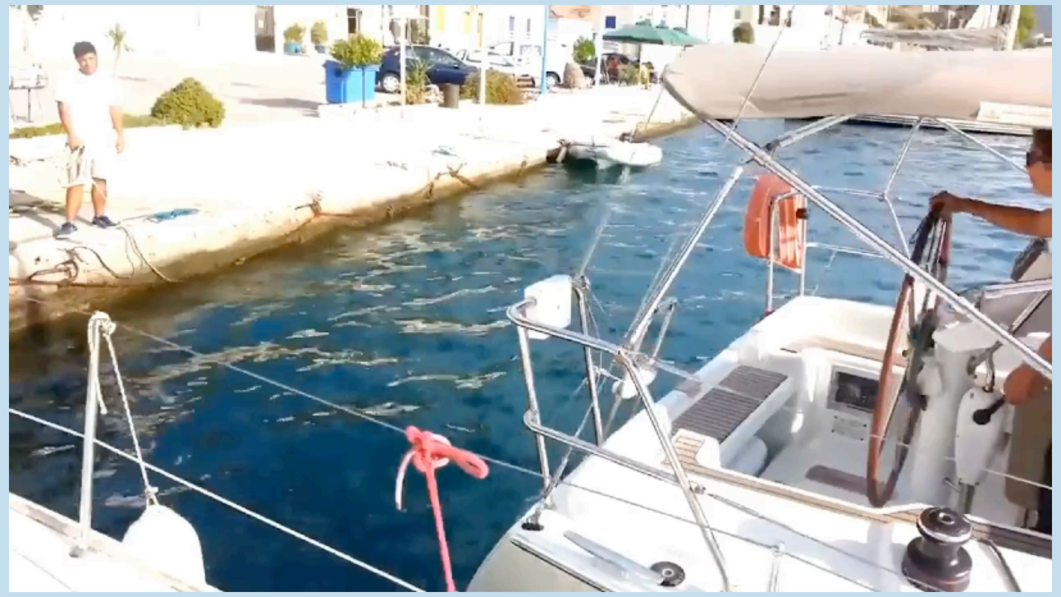

$V_{main}$ 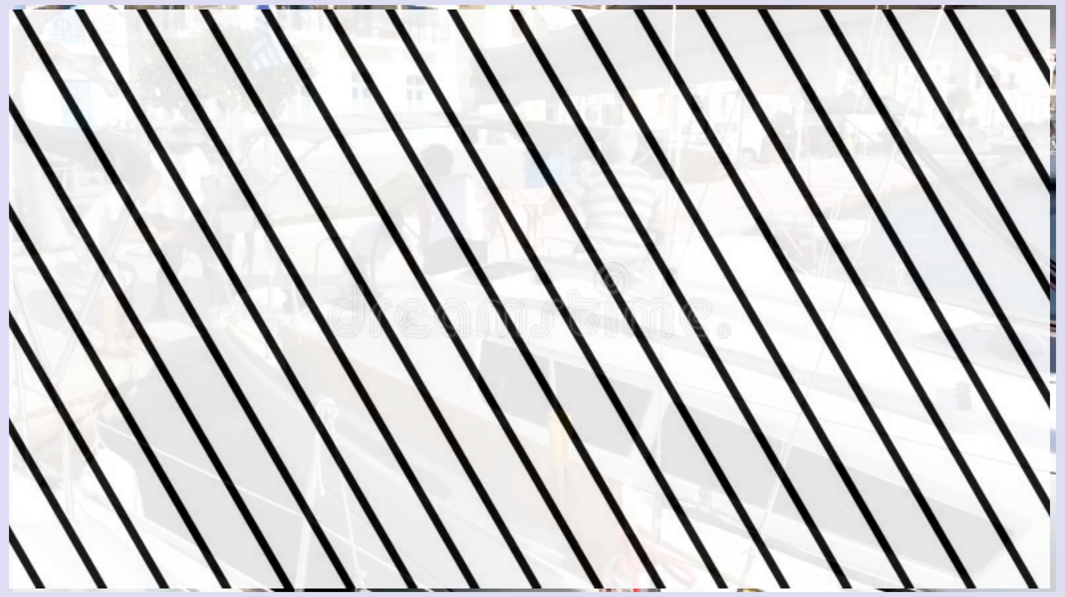

$V_{post}$ 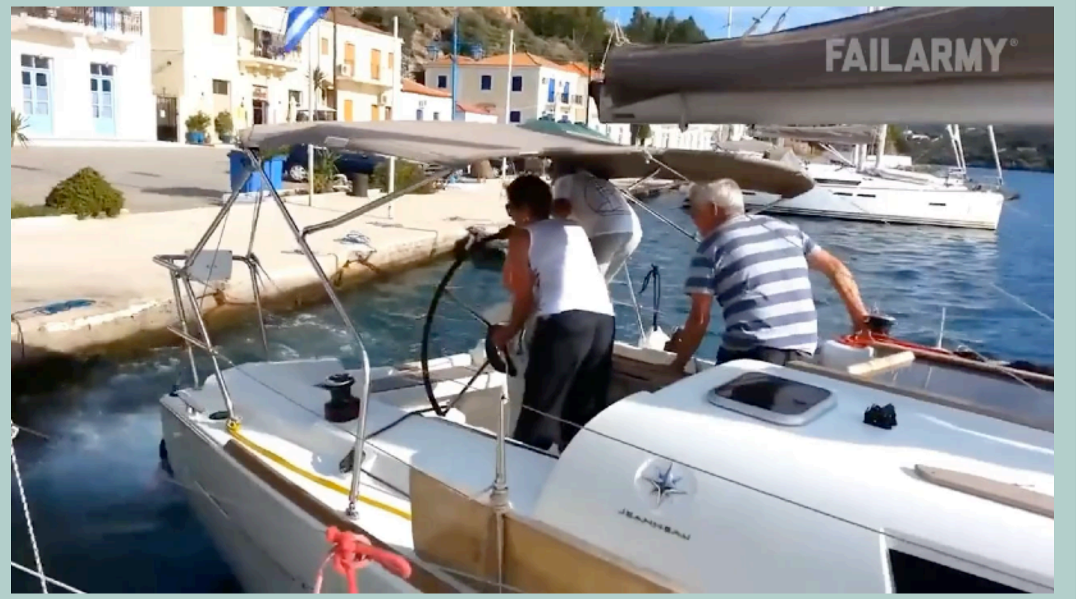


**Question: What could have happened in between?**

A. The man in the striped shirt tries to get off the boat, but falls into the water.
B. The boat ends up drifting backwards and then slams into the dock again.
C. The boat bounces off the dock so hard that it drifts backwards and the men are unable to dock.

**Perception:**

$V_{pre}$**:** A boat is approaching a pier too fast. Two people are on the boat, one is a woman who is attempting to steer the boat and stop it. As the boat is about to collide with the pier three men approach the boat to try to stop it.

$V_{post}$**:** Someone is docking their boat. Someone else is recording on their other boat. The docking boat is going in reverse. An elderly man appears to want to board the other boat, but is stopped.

**Comprehension:**

In the beginning the woman steering the boat tries to slow it down before it hits the dock. The men standing on the dock immediately try to kick the boat to slow it down and push it back. The end video only shows the couple on the boat going backwards for a few seconds.

**GT Ans:** C

**Baseline:** B ❌ | **+Perception:** C ✅ | **+Perception+Comprehension:** C ✅

$V_{pre}$

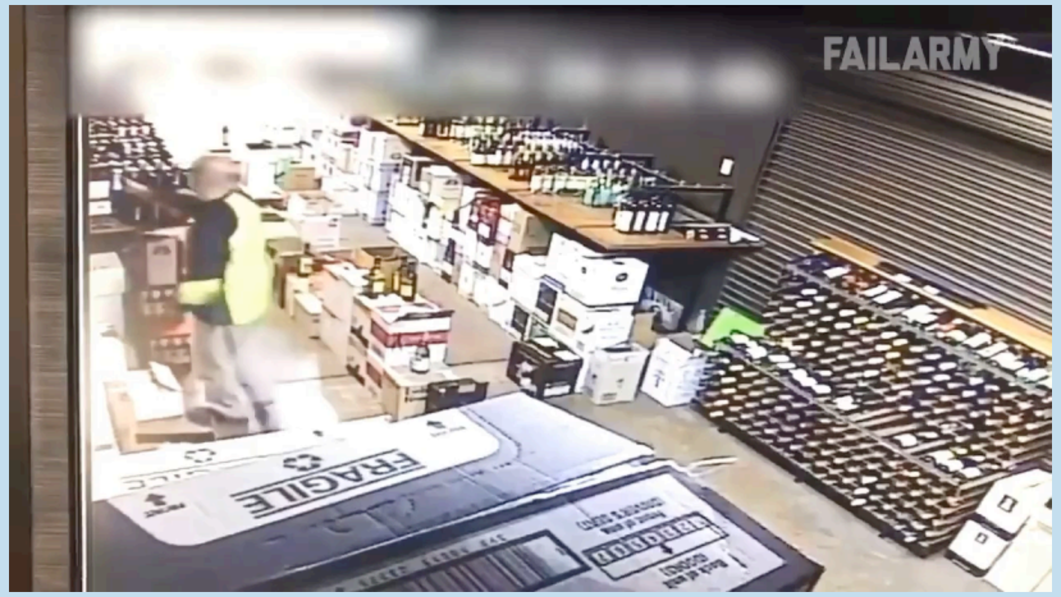


$V_{main}$

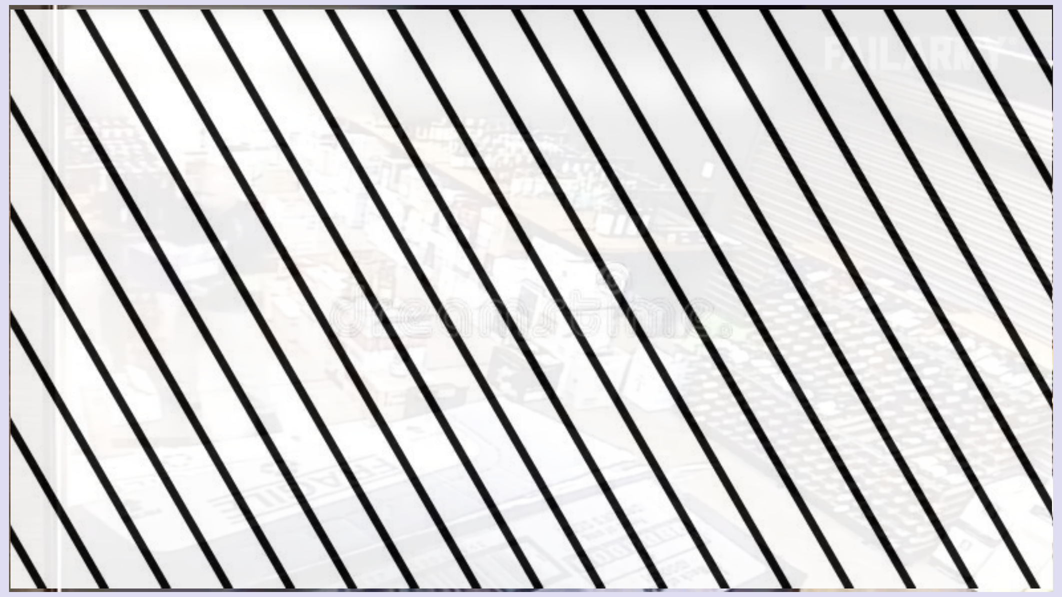

$V_{post}$

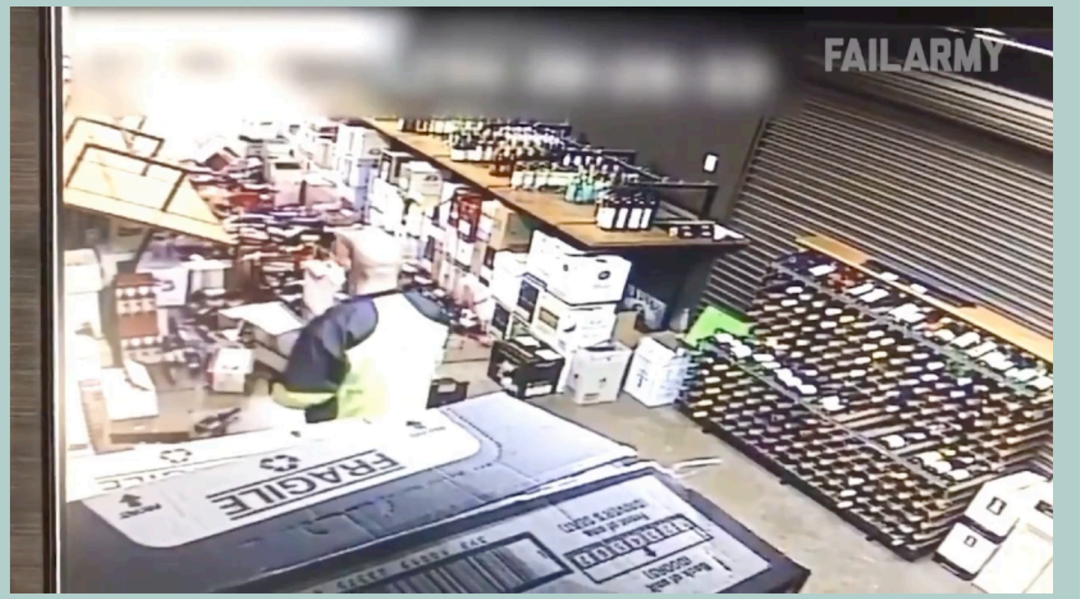


**Question: What could have happened in between?**

A. As the guy carries the box of wine bottles, he begins to slip around while still carrying them.

B. The guy throws the box of wine bottles in the air out of frustration and lets the bottles crash onto the floor all around him.

C. As the man removes a box of wine bottles from the table, the table starts to wobble, causing the other boxes still on the table to start falling to the floor.

**Perception:**

$V_{pre}$: A man is removing a box of wine bottles from a shelf in a liquor storage area or liquor store. The area is closed up and presumably not open to the public or not a retail store.

$V_{post}$: A man is standing with his back to the camera. Surrounding him are many shelves and boxes with what appear to be wine and liquor bores. Directly behind the man is a box labeled "Fragile".

**Comprehension:**

In the beginning, a bald man wearing tan pants, a black shirt, and a yellow vest appears to be taking boxes off a shelf on the left-side wall of a warehouse or brewery. In end, the man is seen facing away from the camera looking at the shelf he originally took the box from. <u>The shelf appears to have tipped</u>, as it's leaning sideways and its contents are all over the floor.

**GT Ans:** C

**Baseline:** B ❌ | **+Perception:** B ❌ | **+Perception+Comprehension:** C ✅
