# Supplementary material for: Black Swan: Abductive and Defeasible Video Reasoning in Unpredictable Events
Source: arXiv:2412.05725 source file (2025-04-07)
Supplement: Supplementary file 4 [file Templates-crop.pdf]

Welcome!

Welcome to this task! Please begin by reading the full instructions and the guidelines.

Full Instructions

[\(Expand/Collapse\)](#)

# Task Instructions

Thanks for participating in this HIT! In this task, you will evaluate an inference derived from a part of a video. Each video is divided into three parts Part 1, Part 2 and Part 3, described below.

- Part 1:** The beginning or setup of the scene in the video.

**Part 2:** The interesting event in the video.

**Part 3:** The result or outcome of the event in the video.

In this task, you will watch only **Part 1** of the video, and **Part 2** and **Part 3** will be hidden. You need to evaluate a description that answers the question, "What could have happened in **Part 2** (the middle part) after seeing Part 1?" based on the criteria listed below. Please refer to the example to understand the scoring better.

## Criteria:

- Correctness (5 Point Scale)** Check whether the answer correctly describes what could have happened in part 2 based on part 1.
- Depth and Thoughtfulness (5 Point Scale)** How much depth in reasoning is covered in the description? Is there sufficient reasoning to support the description?
- Level of Detail (5 Point Scale)** Does the description have sufficient level of detail to easily identify and differentiate between people/objects and actions?
- Visual Contradiction (Yes/No)** Does the description follow the content in the video, or contradict the contents of the video? A contradiction happens when the description is impossible, given the video.

# Example

Given Part 1, what happens next? (in Part 2)

Part 1:

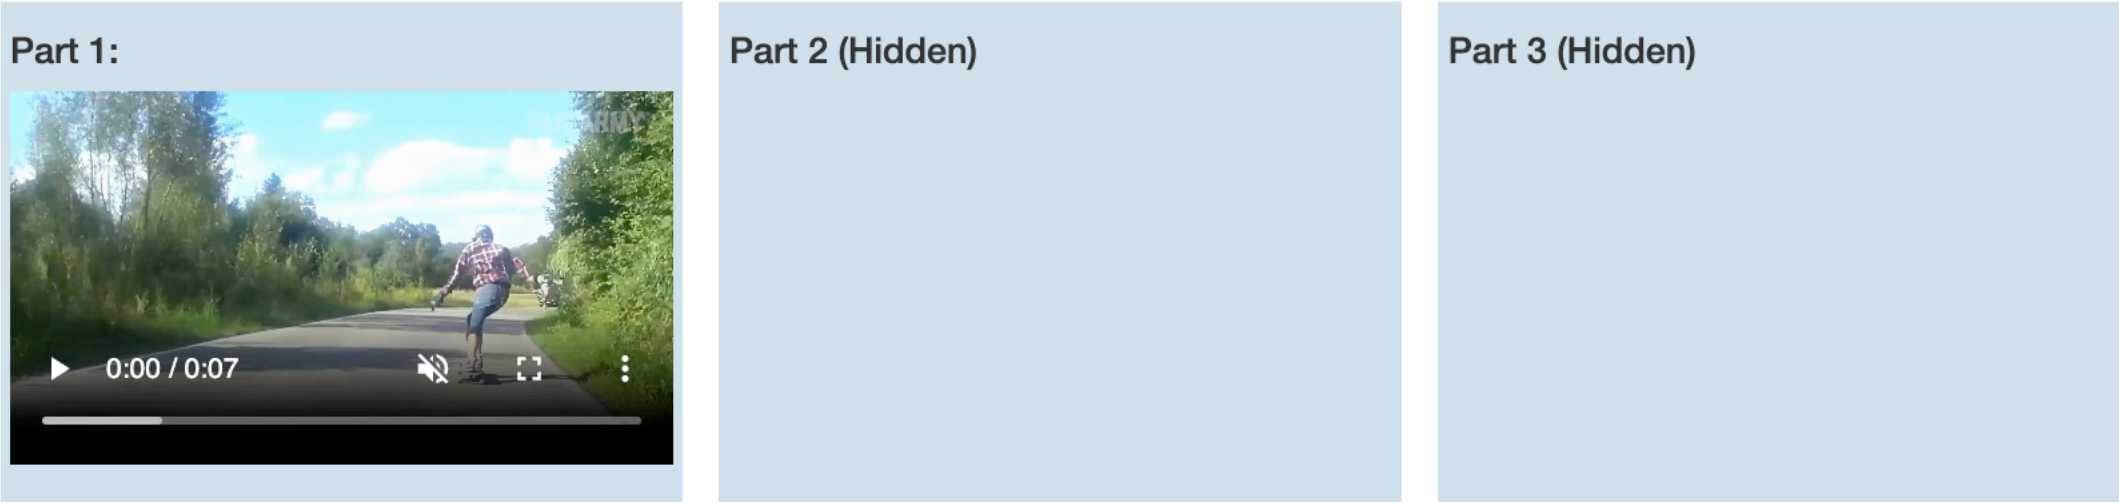

Part 2 (Hidden)

Part 3 (Hidden)

Correctness:

| Description                                                                                                                  | Score | Rubric                | Reason                                                                             |
|------------------------------------------------------------------------------------------------------------------------------|-------|-----------------------|------------------------------------------------------------------------------------|
| The skateboarder in the back goes very close to the one in the front, and it looks like they might collide and lose balance. | 5     | Very likely correct   | Matches the situation well, and the inference is valid based on the video context. |
| The car passes by, and the skateboarder in the back gets too close to the one in the front. There might be an accident.      | 4     | Mostly correct        | Mostly correct but lacks clear mention of balance or specific consequences.        |
| The skateboarder in the back skates faster and overtakes the one in the front. It could lead to a fall.                      | 3     | Partly incorrect      | Partially accurate; overtaking is not visible, but inferring a fall is plausible.  |
| The skateboarder in the back is far away from the front one and continues skating without any issues.                        | 2     | Possibly incorrect    | Incorrect inference; the video shows the skateboarders close to each other.        |
| The skateboarders stop skating and start walking after the car passes by.                                                    | 1     | Very likely incorrect | Completely incorrect as it contradicts the visible actions in the video.           |

Depth and Thoughtfulness:

| Description                                                                                                                                                                                            | Score | Rubric                                     | Reason                                                                                   |
|--------------------------------------------------------------------------------------------------------------------------------------------------------------------------------------------------------|-------|--------------------------------------------|------------------------------------------------------------------------------------------|
| The skateboarder in the back seems to miscalculate the speed and distance from the front skateboarder after the car passes. This could lead to a loss of balance, especially as the road seems narrow. | 5     | Very thoughtful reasoning                  | Thorough and thoughtful with specific details about speed, distance, and road condition. |
| The skateboarder in the back almost collides with the one in the front, which could lead to them both falling.                                                                                         | 4     | Thoughtfully written, but could be better. | Thoughtful, but missing some details like the speed or the road condition.               |
| The skateboarders are skating close to each other, and the one in the back might fall if they collide.                                                                                                 | 3     | Mediocre level of reasoning depth          | Provides some thought but lacks depth or meaningful insight.                             |
| The skateboarder in the back gets very close to the front one, and something bad might happen.                                                                                                         | 2     | Somewhat vague reasoning                   | Too vague and lacks meaningful analysis or details.                                      |
| Both skateboarders keep skating without any issues after the car passes.                                                                                                                               | 1     | No depth in reasoning                      | No depth or thought in the inference; it's a basic and shallow observation.              |

Level of Detail:

| Description                                                                                                                                                | Score | Rubric                                                                                                                            | Reason                                                                                                                                                                 |
|------------------------------------------------------------------------------------------------------------------------------------------------------------|-------|-----------------------------------------------------------------------------------------------------------------------------------|------------------------------------------------------------------------------------------------------------------------------------------------------------------------|
| The skateboarder in the red checkered shirt miscalculates the distance and falls to the grass ahead of him while trying to avoid hitting the one in front. | 5     | The level of detail is sufficient to perfectly identify the people, objects and cause of actions.                                 | "skateboarder in the red checkered shirt" has enough level of detail to differentiate between the two skateboarders and the cause is specifically written.             |
| The skateboarder in the back of the other skateboarder slows down but loses control and falls on the grass.                                                | 4     | The level of detail is good enough to identify the people, objects and cause of actions, but may not be specific in some aspects. | "skateboarder in the back" has enough level of detail to differentiate between the two skateboarders, but additional information like "grass ahead of him" could help. |
| One of the skateboarders slows down but loses control, hits the other skateboarder, and falls on the grass.                                                | 3     | Level of detail may be just sufficient for answering the question.                                                                | "One of the skateboarders" implies that there are two skateboarders, but is not enough level of detail to differentiate between the skateboarders clearly.             |
| The young skateboarder is full of energy, and is going really fast on the roads, but accidentally veers off the road and falls.                            | 2     | Poor level of detail, missing important aspects to differentiate between different people/objects and actions.                    | "young" and "full of energy" are not really important for differentiating between the two skateboarders, in fact, there is no mention of the other skateboarder        |
| A skateboarder hits another skateboarder.                                                                                                                  | 1     | Very poor level of detail. Does not describe the people/objects or actions sufficiently.                                          | Does not differentiate between the skateboarders and does not describe the cause of the fall.                                                                          |

Please keep in mind that the level of detail is specific to the video. For example, in a video where there is only one person, a detailed descripton may only contain "The person" as that is sufficient information.

Visual Contradiction:

| Description                                                                                     | Does the description reasonably follow or contradict what is happening in the video? |
|-------------------------------------------------------------------------------------------------|--------------------------------------------------------------------------------------|
| The skateboarder in the back is close to the front one, and it seems likely they might collide. | Follow                                                                               |
| The car passes, and the skateboarders are close to each other; a collision might occur.         | Follow                                                                               |
| The skateboarders are far apart from each other, and no collision seems possible.               | Contradict                                                                           |
| The skateboarders suddenly stop and walk away from the scene.                                   | Contradict                                                                           |

Given Part 1, what happens next? Validate this answer.

Part 1:

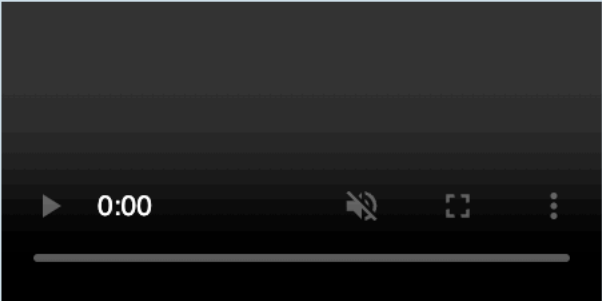

Part 2 (Hidden)

Part 3 (Hidden)

Here is an answer that describes "What happens next (in Part 2)?"

[[task.row\_data['reference\_text']]]

Evaluate the description (in green) based on the below criteria:

1. Correctness (Rate 1-5):

Does the description (in green) correctly answer the question (in red)?

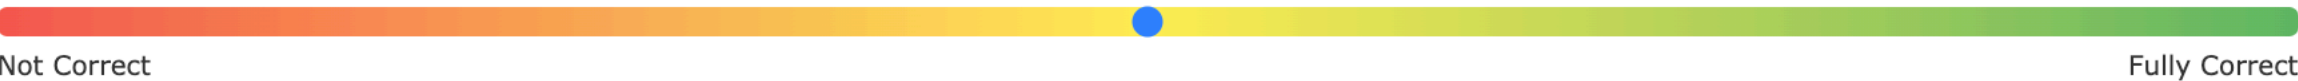

Score: 3

Please explain why you rated this score:

2. Depth and Thoughtfulness (Rate 1-5):

How much depth in reasoning is covered in the description? Is there sufficient reasoning to support the description?

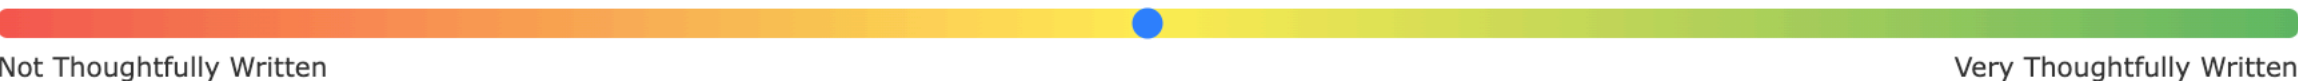

Score: 3

Please explain why you rated this score:

3. Level of Detail (Rate 1-5):

Does the description have sufficient level of detail to easily identify and differentiate between people/objects and actions?

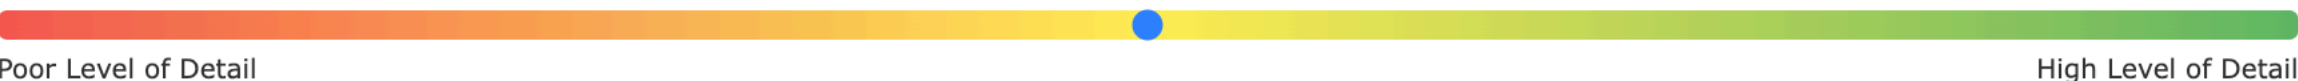

Score: 3

Please explain why you rated this score:

4. Visual Contradiction:

Does the description reasonably follow or contradict what is happening in the video?  
A description is a contradiction only if it is impossible for that scenario to happen, based on Part 1.

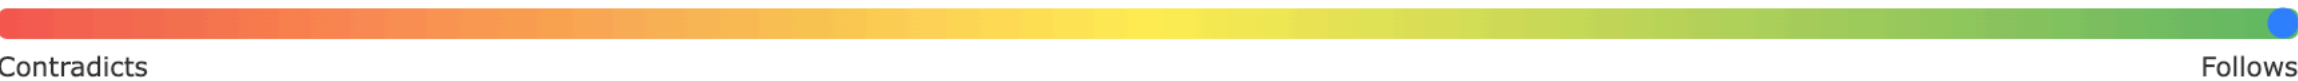

Please explain why you rated this score:

☐ Optional Feedback: Something about the HIT is unclear/These videos have hateful/offensive content/You have additional feedback:

Submit



# Task Instructions

Thanks for participating in this HIT! Each video is divided into three parts Part 1, Part 2 and Part 3, described below.

- Part 1:** The beginning or setup of the scene in the video.
- Part 2:** The interesting event in the video.
- Part 3:** The result or outcome of the event in the video.

## Tasks:

1. **Task 1:** First, you will watch **Part 1** of the video, and **Part 2** and **Part 3** will be hidden. You need to write **diverse** descriptions of what could have happened in **Part 2** (the middle part).
2. **Task 2:** Next, you will be revealed **Part 3** of the video. You need to validate whether your descptions from Task 1 can answer the question *What happens in between **Part 1** and **Part 3*** ?. If marked invalid, you **must** update a new one based on the video. Update descriptions for any changes, even if they are **minor**.
3. **Task 3:** Finally, you will get to watch **Part 2** in the video. Evaluate if any of your previous descriptions align with **all three parts of the video**. You also need to provide a new description, based on the ground truth video shown to you.

In all the tasks, please make sure your descriptions capture the *visual* context in the video accurately. As we provide more visual context and expose you to additional parts of the video, we expect more and more visually grounded descriptions.

# Example

## Task 1: Given Part 1, guess Part 2

Part 1:

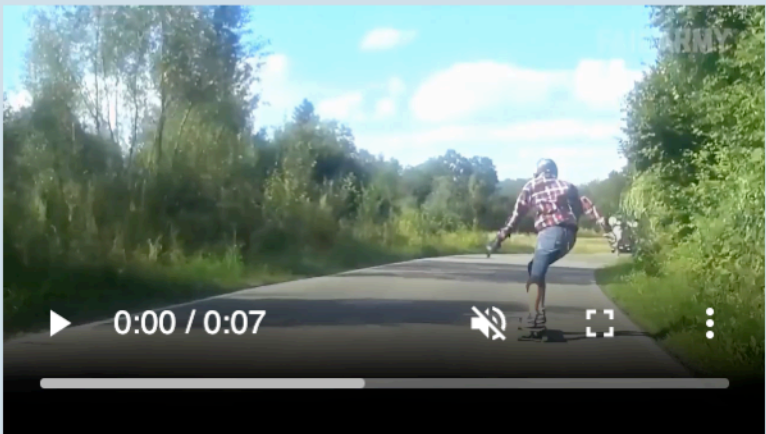

Part 2 (Hidden)

Part 3 (Hidden)

Think about what could happen in Part 3 (the outcome of the video).  
Write three possible descriptions on what will happen in Part 2 to lead to any outcome in Part 3.

1. The skateboarder in the back hits the person skating in the front and they both lose balance.
2. The skateboarder in the back moves closer to the person skating in front but goes around him, avoiding an accident.
3. The skateboarder in the back hits the person skating in the front, and they both hit a car.

## Task 2: Given Part 1 & 3, update Part 2

Part 1:

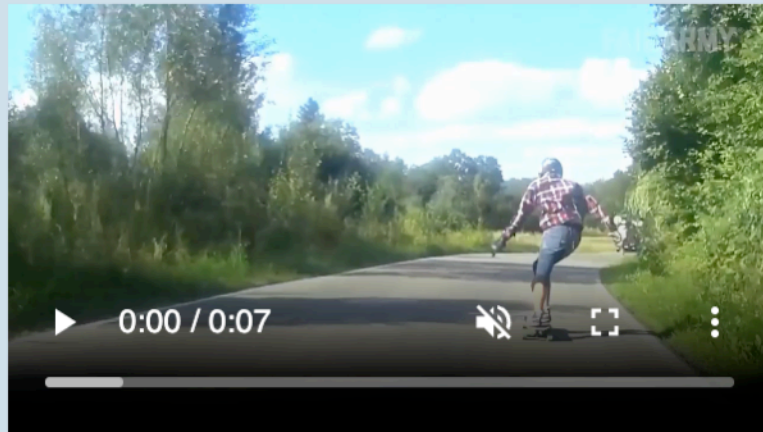

Part 2 (Hidden)

Part 3:

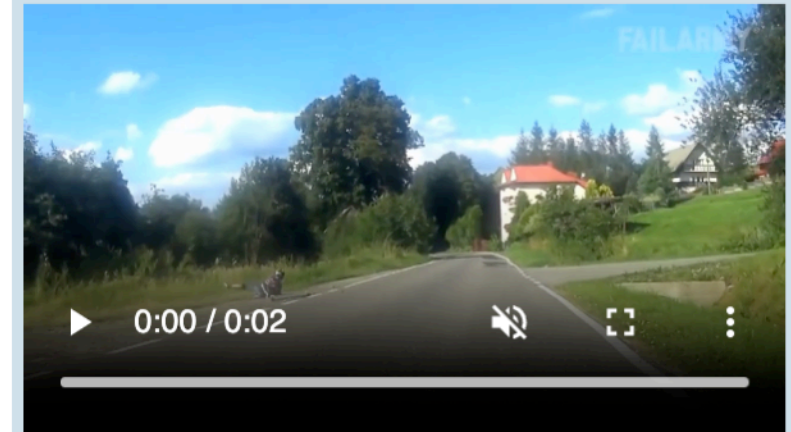

After watching Part 3, you need to update your descriptions for Part 2.

Validate what could have happened in this part.

Please write a new description for each invalid one.

- Description:* The skateboarder in the back hits the person skating in the front and they both lose balance.

✓ Valid
- Description:* The skateboarder in the back moves closer to the person skating in front but goes around him, avoiding an accident.

✗ Invalid (the skateboarder does fall)

*Updated Description:* The skateboarder in the back tried to go around the skateboarder in front, but he still lost balance and fell on the roadside.
- Description:* The skateboarder in the back hits the person skating in the front, and they both hit a car.

✗ Invalid (There is no car)

*Updated Description:* The skateboarder in the back hits the person skating in the front causing him to turn and fall in the middle of the road.

## Task 3: Given all parts, validate Part 2

Part 1:

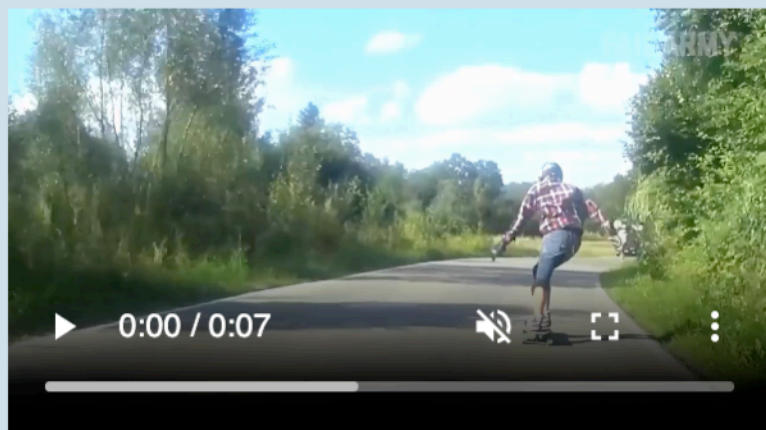

Part 2:

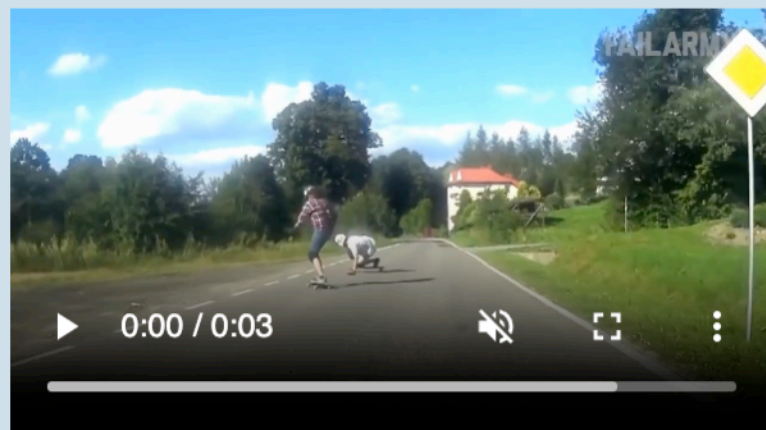

Part 3:

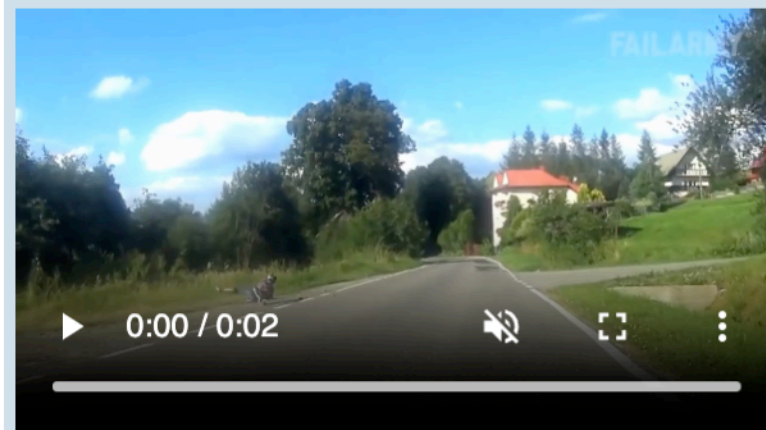

Select the valid descriptions for this part. If none are valid, please write a new description.

1. *Description:* The skateboarder in the back hits the person skating in the front and they both lose balance.  
☐ Invalid (the skateboarder in the front does not lose balance/fall.)
2. *Description:* The skateboarder in the back tried to go around the skateboarder in front, but he still lost balance and fell on the roadside.  
☒ Valid
3. *Description:* The skateboarder in the back hits the person skating in the front causing him to turn and fall in the middle of the road.  
☐ Invalid (the skateboarder in the front does not get hit by the skateboarder in the back.)

## Guidelines:

- **Visually grounded** - Your descriptions should be grounded to the visual context - objects, scenes and activities in the video.
- **Plausible** - Your descriptions should be plausible. Please don't write descriptions that break physical rules or are against common sense.
- **Persuasive** - Your descriptions should be persuasive. It should add sufficient information so that the outcome happened given the initial context of the video.
- **Non-contradictory** - Do not contradict the information in the videos.



# Task 1: Given Part 1, describe Part 2

Part 1:

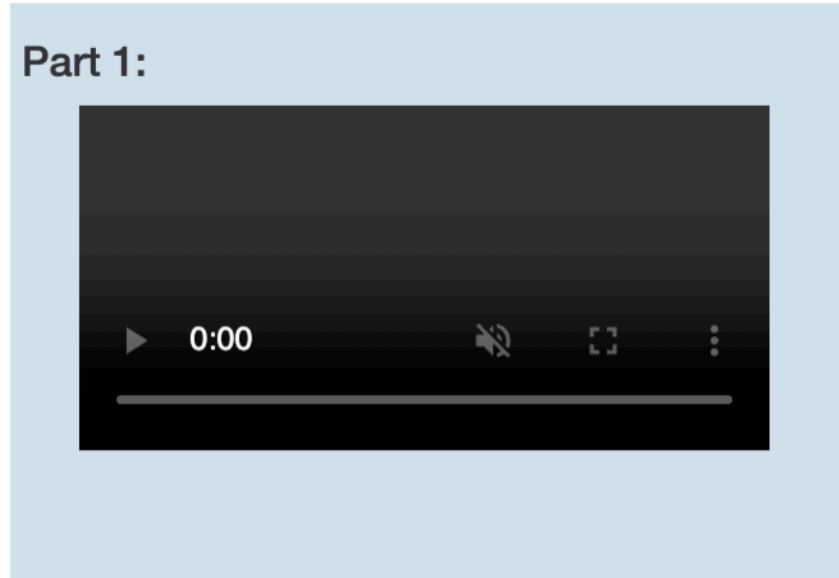

Part 2 (Hidden)

Part 3 (Hidden)

Think about what could happen in Part 3 (the outcome of the video).

**Write three possible diverse descriptions on what will happen in Part 2 to lead to any outcome in Part 3.**

Describe WHY and HOW (rationale) to reach Part 3.

Describe WHY and HOW (rationale) to reach Part 3.

Describe WHY and HOW (rationale) to reach Part 3.

Please write at least 8 words per description. All descriptions should be unique. Please avoid using "it", "he", "she" or "they"; instead use specific descriptions like "the cat" or "the boy on the skateboard".

Think about what could happen in the outcome here!

You should consider many possible outcomes, then write the descriptions in Part 2.

For an example of how each part looks, please see the instructions above.

Please check that your descriptions are:

- Visually grounded
- Plausible
- Persuasive
- Non-contradictory

Proceed to Task 2

# Task 2: Given Part 1 & 3, describe Part 2

Part 1:

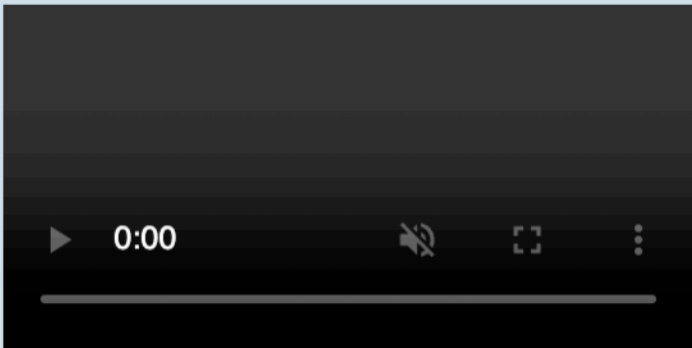

Part 2 (Hidden)

Part 3:

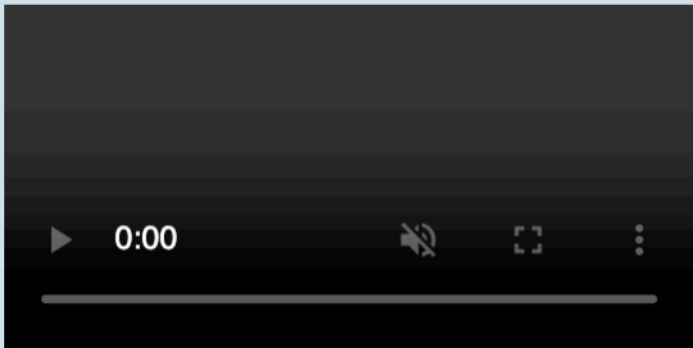

After watching Part 3, are your answers from Task 1 still possible?

Previous:  
Is this description still possible?

- ☒ Yes, possible
- ☐ No, impossible

Previous:  
Is this description still possible?

- ☒ Yes, possible
- ☐ No, impossible

Previous:  
Is this description still possible?

- ☐ Yes, possible
- ☒ No, impossible

Please write a new description to replace the impossible ones. No duplicates please, you can be creative!

Describe what could happen in Part 2 to lead to Part 3

Please write at least 8 words per new description. Also, do NOT describe the outcome of the event that you see in Part 3; only write about Part 2.

Please check that your descriptions are:

- Visually grounded
- Plausible
- Persuasive
- Non-contradictory

Proceed to Task 3



# Task 3: Given all parts, validate Part 2

Part 1:

▶ 0:00 🔊 📺 ⋮

Part 2:

▶ 0:00 🔊 📺 ⋮

Part 3:

▶ 0:00 🔊 📺 ⋮

Select the description, that are correct/possible after watching the video.

Previous:  
Is this description still correct/possible?

- ☐ Yes, possible
- ☐ No, impossible

Previous:  
Is this description still correct/possible?

- ☐ Yes, possible
- ☐ No, impossible

Previous:  
Is this description still correct/possible?

- ☐ Yes, possible
- ☐ No, impossible

Finally, please write a new description based on the true video. Make sure your description is specific and detailed, and accurately describes the events in Part 2 and Part 3:

Final detailed description. Be more specific and accurate than your previous descriptions.

Required Feedback: Are there more than one complete events/clips/videos in the video (*spanning Part 1, 2 & 3*).

- ☐ Yes
- ☐ No

[In general, this should be "No", but if you find a case where there are two complete sub-videos in one video, please report "Yes" here.]

Please check that your descriptions are:

Visually grounded

Plausible

Persuasive

Non-contradictory

☐ Optional Feedback: Something about the HIT is unclear/These videos have hateful/offensive content/You have additional feedback:

Submit

Welcome!

Welcome to this task! Your goal is to watch the provided videos and choose the most accurate option from the given set of options.

Full Instructions (Expand/Collapse)

## Task Instructions

Thanks for participating in this HIT! This is a task where you will look at videos and choose the right option for the given question.

Guidelines:

- Please read the options carefully.
- Please watch the video(s) completely.
- Be as reasonable as you can, and make a smart guess if you are unsure.

## Task: Multiple Choice Question Answering

Part 1:

0:00

Part 2 (Hidden)

Part 3

0:00

**Question: Which of the following could have happened in between the two videos (in Part 2) shown here?**

If no option seems correct, pick the most plausible (but not impossible) option.

- ☐ \${option1}
- ☐ \${option2}
- ☐ \${option3}

Please read all options carefully, as the options may vary in very specific ways.

Submit

Welcome!

Welcome to this task! Your goal is to watch the provided videos and choose the most accurate option from the given set of options.

Full Instructions (Expand/Collapse)

## Task Instructions

Thanks for participating in this HIT! This is a task where you will look at videos, read a hypothesis, and choose the right option for the given question.

Guidelines:

- Please read the hypothesis carefully.
- Please watch the video(s) completely.
- Be as reasonable as you can, and make a smart guess if you are unsure.

## Task: Multiple Choice Question Answering

Part 1:

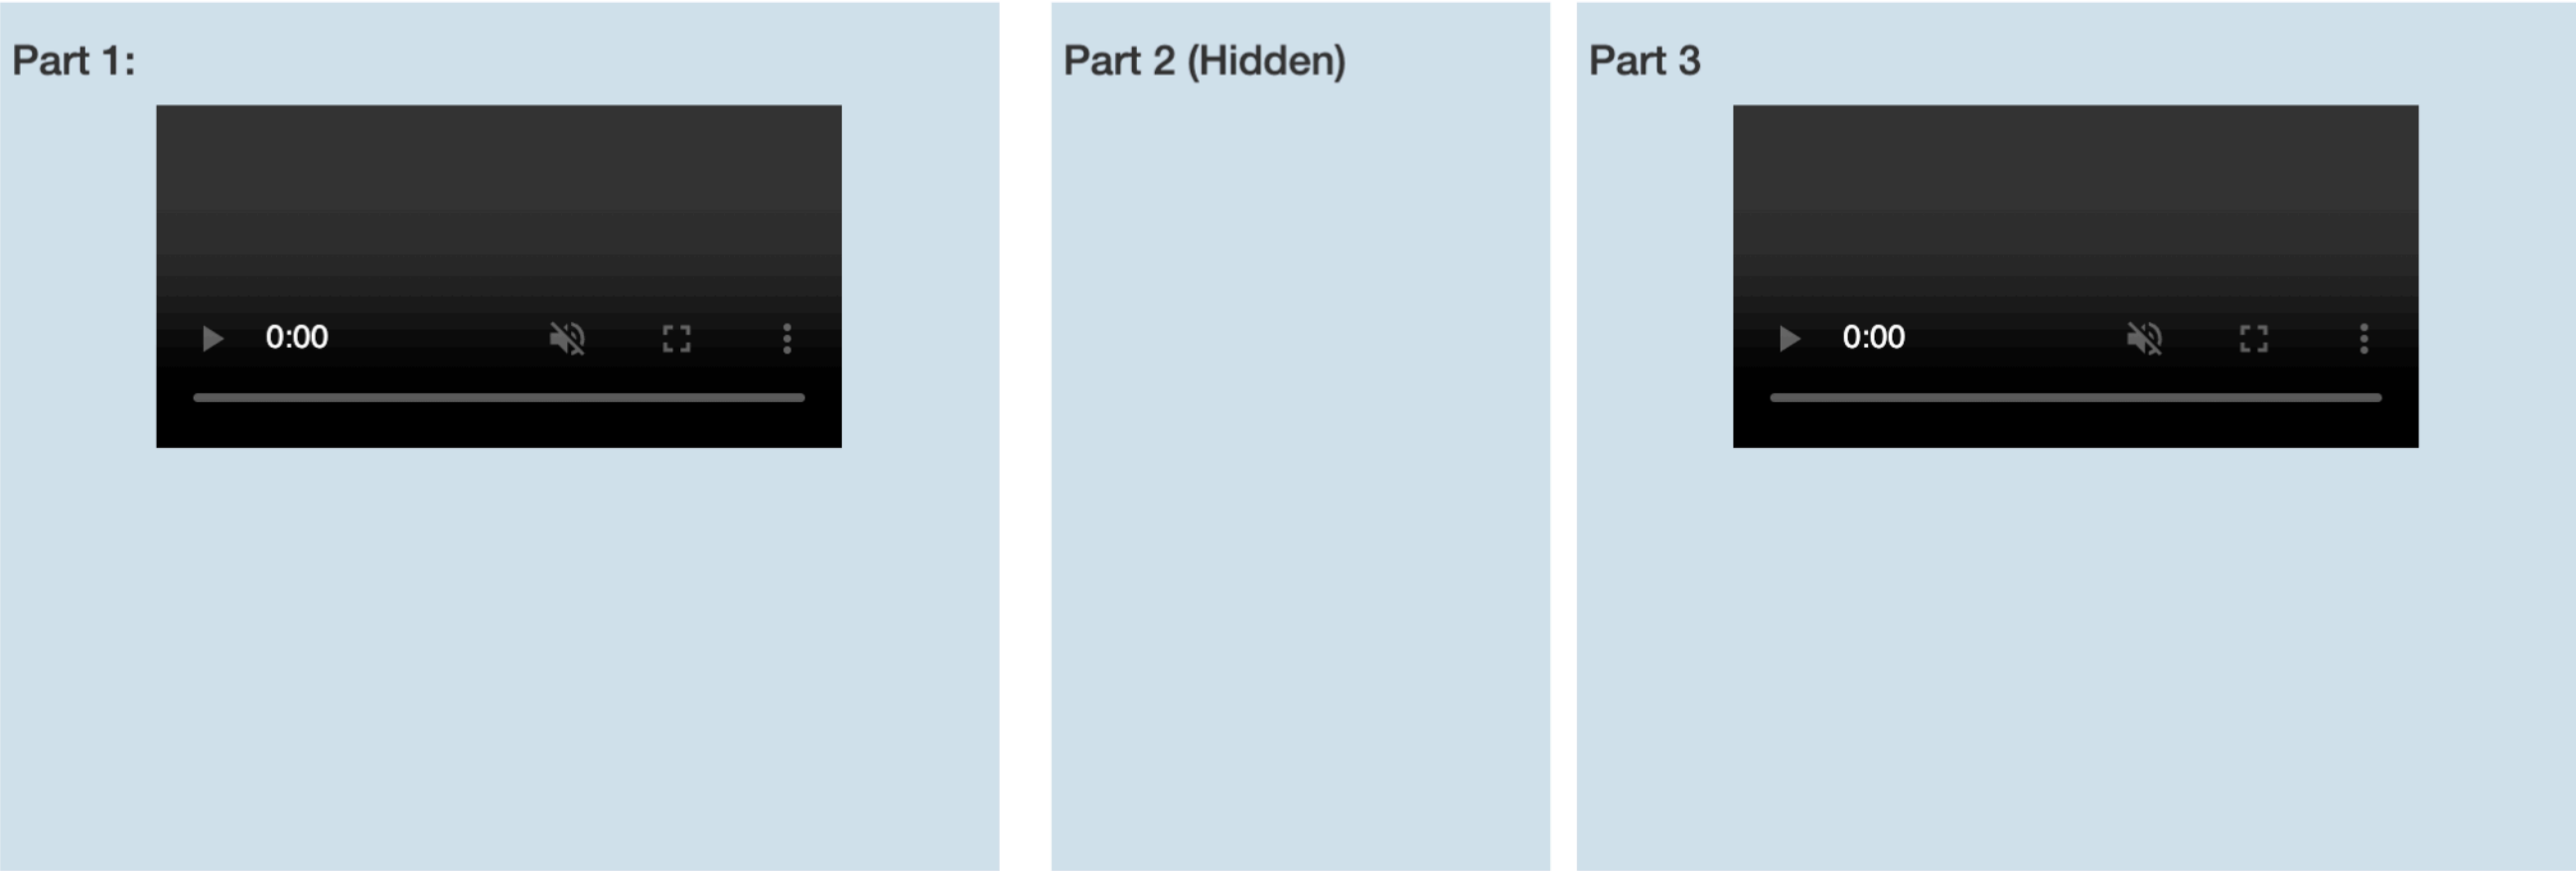

Part 2 (Hidden)

Part 3

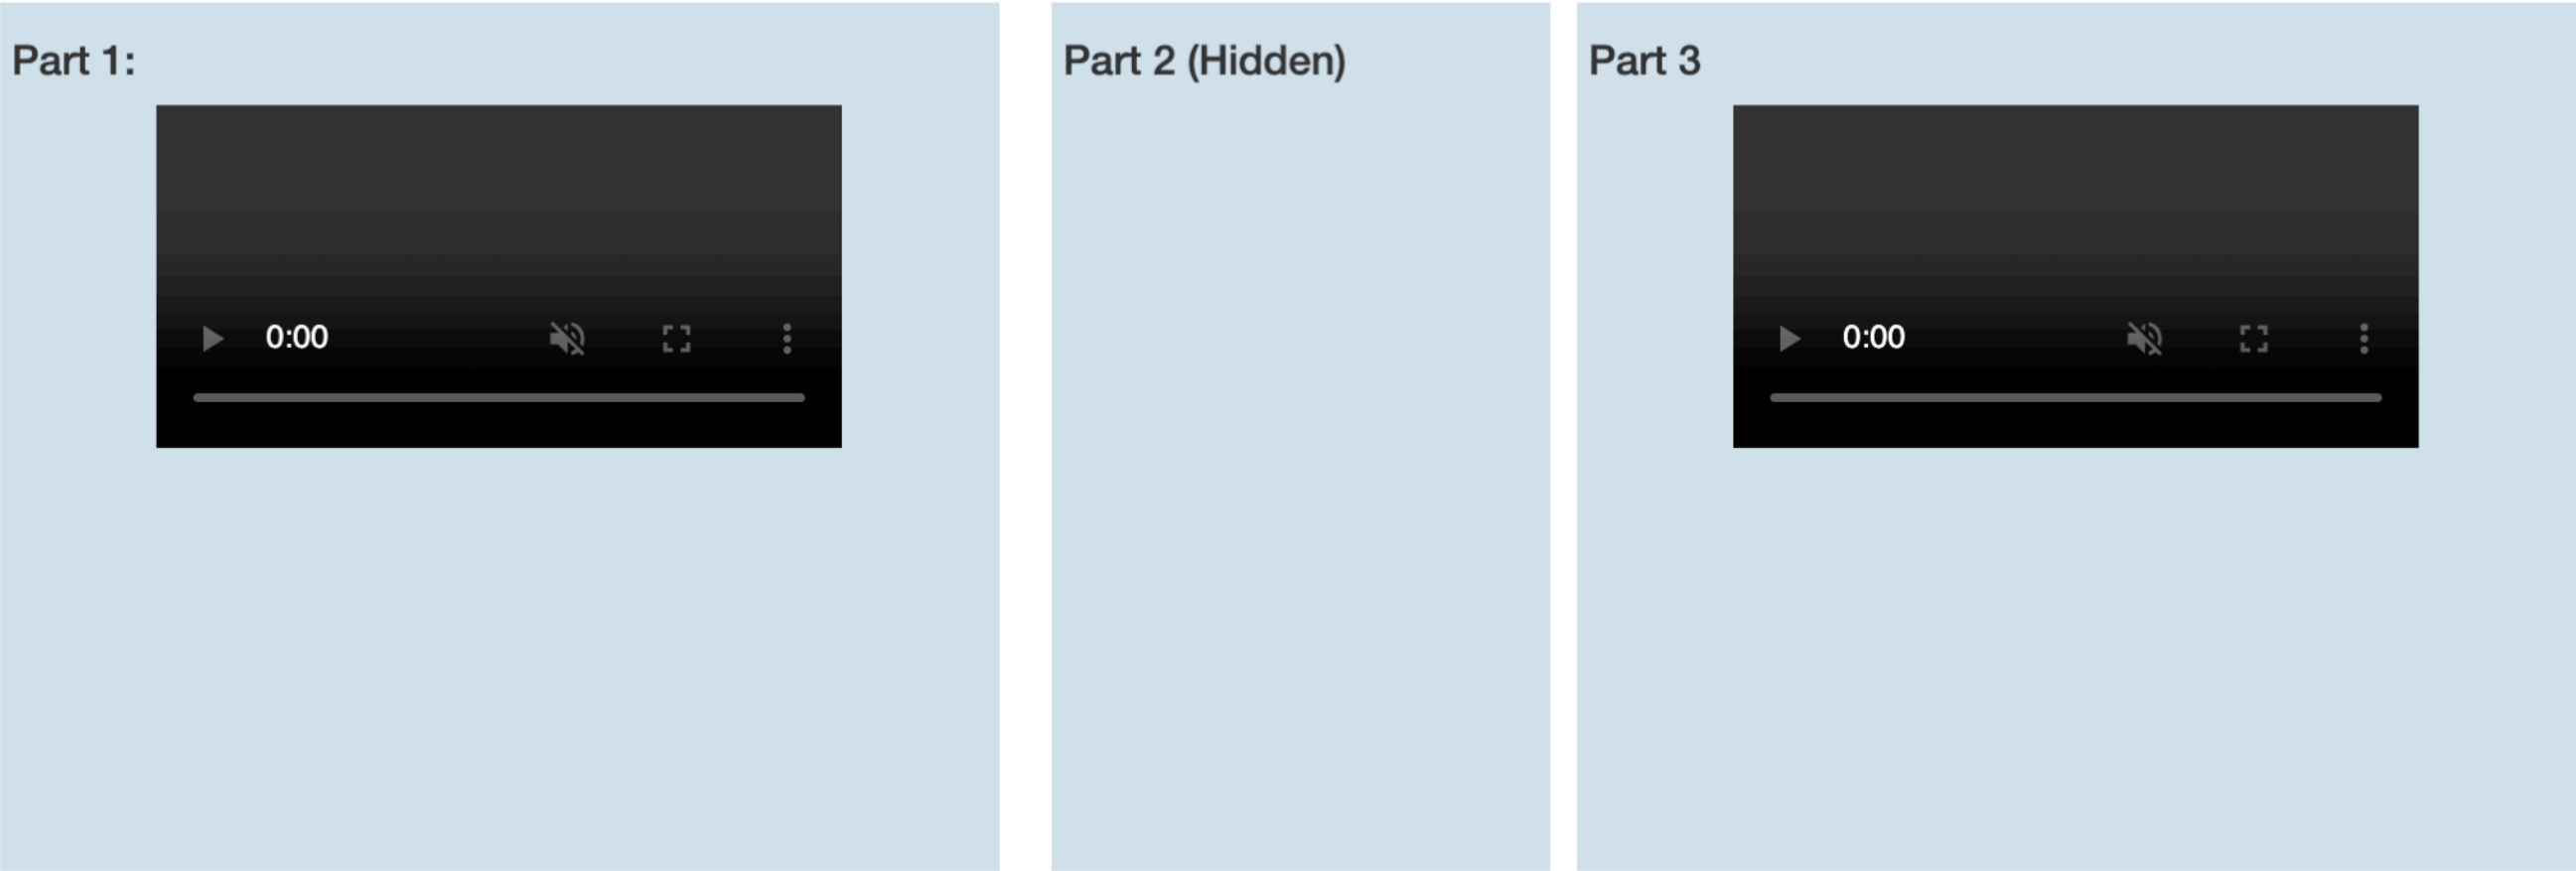

Hypothesis: {{ task.row\_data['exp'] }}

Question: Given the beginning and end of a video, does this hypothesis hold?

Please watch the video carefully before answering.

☐ Yes

☐ No

Submit



Instructions

Welcome to this task! Please read the question carefully and answer it. All parts must be completed before submitting.

Given the beginning of a video, what what could happen next?

Beginning:

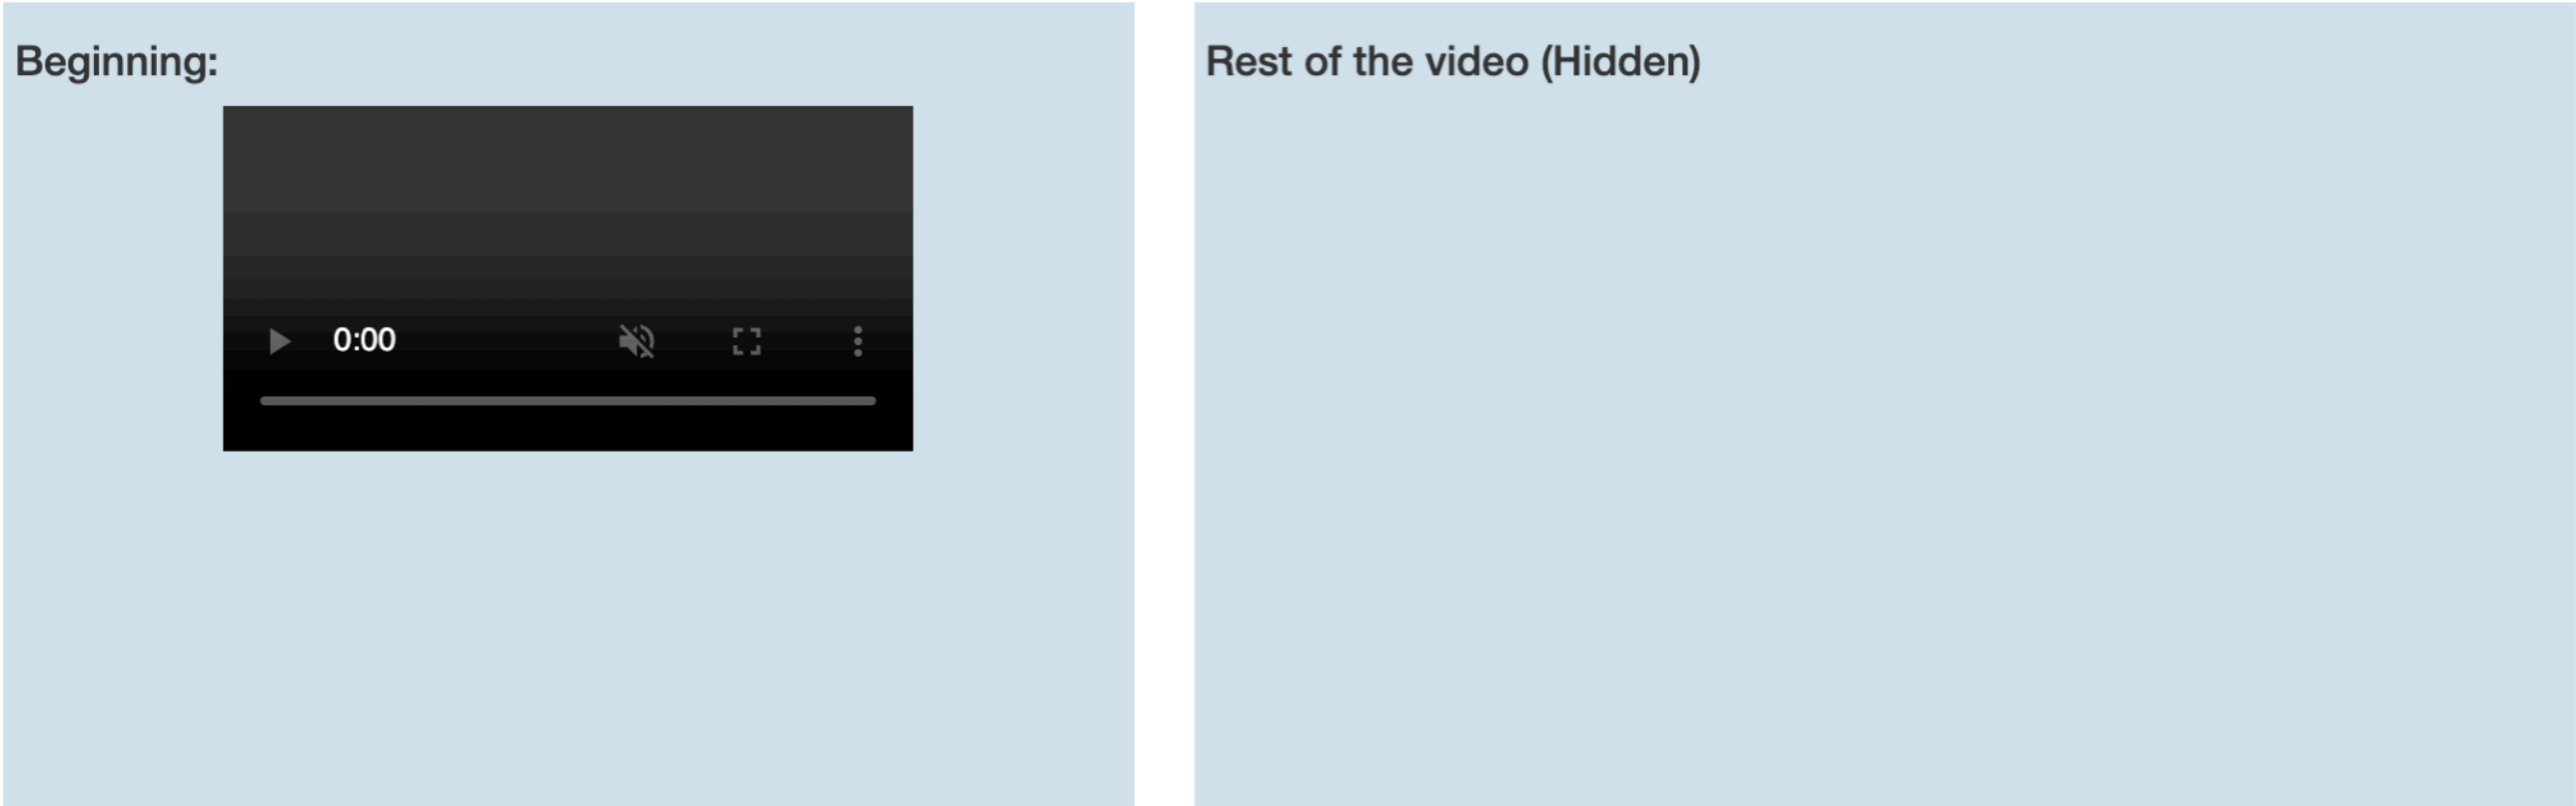

Rest of the video (Hidden)

**Explain what will happen next.**  
**Write three possible diverse explanantions:**

What happens next? Also describe WHY and HOW (rationale).

What happens next? Also describe WHY and HOW (rationale).

What happens next? Also describe WHY and HOW (rationale).

Please write at least 8 words per description. All explanations should be unique. Please avoid using "it", "he", "she" or "they"; instead use specific descriptions like "the cat" or "the boy on the skateboard".

☐ *Optional Feedback:* Something about the HIT is unclear/These videos have hateful/offensive content/You have additional feedback:

Submit
